# Supplementary material for: Let's Negotiate! A Survey of Negotiation Dialogue Systems
Source: arXiv:2402.01097 source file (2024-02-02)
Supplement: Supplementary file 1 [file 12_appendix.tex]

\section{Literature Curation}

In this section, we provide details about how the literature was curated for our survey. We hope this helps the overall reproducibility and also guides similar studies in the future. We followed a simple
two-stage process. First, we investigated the relevant datasets that capture various forms of negotiation across diverse domains (presented in Section 4) and then, we surveyed the methods developed
on these datasets (presented in Section 3).

We investigated the past 10 years of *ACL conference proceedings.

\section{Related Surveys}

\section{Appendix}

\paragraph{Decoupling Strategy and Generation in Negotiation Dialogues \cite{he2018decoupling}}
\begin{itemize}
\item They collected negotiation dialogues dataset named CraigslistBargain, which is available here \footnote{\url{https://stanfordnlp.github.io/cocoa/}}. Comparing to other dataset, CraigslistBargain is designed to focus on more realistic scenarios. During data collection, two agents are assigned the role of a buyer and a seller; they are required to negotiate the price of a given item. As the real scenario, the listing price is available to both sides, but buyer has a private price as target. Then two agents chat freely to decide the final price. When a price is accepted  by the partner, the task is completed. Agents can also quit the conversation as no agreement completion. Furthermore, agents can negotiate side offers (e.g. free delivery or pick up) to simulate real scenarios. Statistics of CraigslistBargain are shown in Table~\ref{tab:CraigslistBargain_statistics}.
\item They define coarse dialogue acts (e.g. greet, disagree, insist, inquire, propose, counter, etc), which serves as a logical skeleton on conversation level. Each utterance is assigned with one dialogue act.
\item The proposed model contains three modules: a parser that maps an utterance into dialogue act; a manager that predict next dialogue act given past history; a generator that produce natural language response conditioning on past history and predicted dialogue act.
\end{itemize}

\begin{table}[t]
\begin{tabular}{ll}
\hline
\# of unqiue posting             & 1402  \\
\% with images                   & 80.8  \\
Avg \# of tokens per description & 42.6  \\
Avg \# of tokens per title       & 33.8  \\
Vocab size                       & 12872 \\
\# of dialogues                  & 6682  \\
Avg \# of turns                  & 9.2   \\
Avg \# of tokens per turn        & 15.5  \\
Vocab size                       & 13928 \\
Vocab size (excl. numbers)       & 11799 \\ \hline
\end{tabular}
\caption{Statistics of CraigslistBargain dataset.}
\label{tab:CraigslistBargain_statistics}
\end{table}

\paragraph{Evaluating and Enhancing the Robustness of Dialogue Systems: A Case Study on a Negotiation Agent \cite{cheng-etal-2019-evaluating}}
This work develops algorithms to evaluate the robustness of negotiation agents via designed adversarial attacks. For example, a negotiation agent is not robust if an adversarial agent can fool the negotiation agent to make a deal against its benefit. They evaluate the negotiation agent developed by \citet{lewis2017deal}. They propose both black-box attack algorithms and white-box attack algorithms. For black-box attack, they propose two algorithms:
\begin{itemize}
\item Reinforcement learning attack: they train adversarial agent by reinforcement learning, where the reward is the difference between adversarial agent's score and target agent's score ($r^{adv}=S_{adv}-S_{ori}$).
\item Transfer attack: they main idea is: a sentence leading to bad deal in one dialogue might also lead to similar results in other dialogues. They collect a list of last sentences $L$ that resulting in bad deal for target agent. In the conversation, they let adversarial agent plug in one sentence from $L$ at the last turn.
\end{itemize}
They also propose two white-box attack algorithms:
\begin{itemize}
\item Reactive attack: the main idea is still guide target agent to make a bad decision that is in favor of the adversarial agent. They formulate this attack as an optimization problem through a designed loss function that is in favor of adversarial agent.
\item Preempative attack: this approach is to produce a sentence that guide target agent to decrease its demand. Similarly, this method can be formulated as an optimization problem through designed loss function.
\end{itemize}
The experiment results show that current negotiation agents are not robust against their adversarial agents. But, by iterating adversarial training, the robustness of the agent can be significantly improved.
